# Supplementary material for: Range (R\'enyi) Entropy Queries and Partitioning
Source: arXiv:2312.15959 source file (2025-10-29)
Supplement: Supplementary file 1 [file appendix.tex]

\appendix
